# Supplementary material for: Symmetry constraints and spectral crossing in a Mott insulator with Green's function zeros
Source: arXiv:2301.13870 ancillary file (2024-06-09)
Supplement: Supplementary file 1 [file Mott_Zeros_SI.pdf]

# Supplemental Material: Symmetry constraints and Spectral crossing in a Mott insulator with Green's function zeros

Chandan Setty[⊕,*,1], Shouvik Sur[†,*,1], Lei Chen[1], Fang Xie[1],
Haoyu Hu[2], Silke Paschen[3,1], Jennifer Cano[4,5], and Qimiao Si[1]
[1]*Department of Physics and Astronomy, Rice Center for Quantum Materials, Rice University, Houston, Texas 77005, USA*
[2]*Donostia International Physics Center, P. Manuel de Lardizabal 4, 20018 Donostia-San Sebastian, Spain*
[3]*Institute of Solid State Physics, Vienna University of Technology, Wiedner Hauptstr. 8-10, 1040, Vienna, Austria*
[4]*Department of Physics and Astronomy, Stony Brook University, Stony Brook, NY 11794, USA and*
[5]*Center for Computational Quantum Physics, Flatiron Institute, New York, NY 10010, USA*

## CONTENTS

I. Square net model 1
A. Minimal interacting model 2
B. Numerical solution for generic interactions 3

II. Green's function 4

III. One-band HK Model 5

IV. Spectral degeneracy enforced by non-symmorphic crystalline symmetry 6

V. Matrix-form of the interacting Green's function 7

VI. Broken time reversal symmetry case 8

VII. Crossings of Green's function zeros for the Hubbard model 9

VIII. Spectral crossings on the diamond lattice 9

References 9

## I. SQUARE NET MODEL

Young and Kane constructed a model of 2D Dirac semimetal on a crinkled checkerboard lattice,

$$\begin{aligned}\tilde{h}_0 &= t_2(\cos k_x + \cos k_y)\mathbb{1} + 2t\cos\frac{k_x}{2}\cos\frac{k_y}{2}\tau_1\otimes\sigma_0 \\ &+ t_{SO}\left[\sin k_x \tau_3\otimes\sigma_2 - \sin k_y \tau_3\otimes\sigma_1\right],\end{aligned} \tag{S1}$$

where $\tau_j$ ($\sigma_j$) is the $j$-th Pauli matrix acting on the sublattice (spin) subspace, and $\mathbb{1}$ is the $4\times 4$ identity matrix. This Hamiltonian can be block-diagonalized as

$$\tilde{h}_0 \to h_0 = e^{i\frac{\pi}{4}\tau_2\otimes\sigma_3}\tilde{h}_0 e^{-i\frac{\pi}{4}\tau_2\otimes\sigma_3}, \tag{S2}$$

with

$$\begin{aligned}h_0 &= t_2(\cos k_x + \cos k_y)\mathbb{1} + 2t\cos\frac{k_x}{2}\cos\frac{k_y}{2}\tau_3\otimes\sigma_3 \\ &+ t_{SO}\left[\sin k_x \tau_3\otimes\sigma_2 - \sin k_y \tau_3\otimes\sigma_1\right].\end{aligned} \tag{S3}$$

We note that the bases for $\tilde{h}_0$ and $h_0$ are, respectively,

$$\tilde{\Phi} = \begin{pmatrix} c_{A,\uparrow} \\ c_{A,\downarrow} \\ c_{B,\uparrow} \\ c_{B,\downarrow} \end{pmatrix}, \quad \Phi = \frac{1}{\sqrt{2}} \begin{pmatrix} c_{A,\uparrow} + c_{B,\uparrow} \\ c_{A,\downarrow} - c_{B,\downarrow} \\ -c_{A,\uparrow} + c_{B,\uparrow} \\ c_{A,\downarrow} + c_{B,\downarrow} \end{pmatrix} \equiv \begin{pmatrix} \phi_{+,\Uparrow} \\ \phi_{+,\Downarrow} \\ \phi_{-,\Uparrow} \\ \phi_{-,\Downarrow} \end{pmatrix}, \tag{S4}$$

where $A$ and $B$ denote the two sublattices of the checkerboard lattice. For our purpose, it is convenient to set $t_2 = 0$.

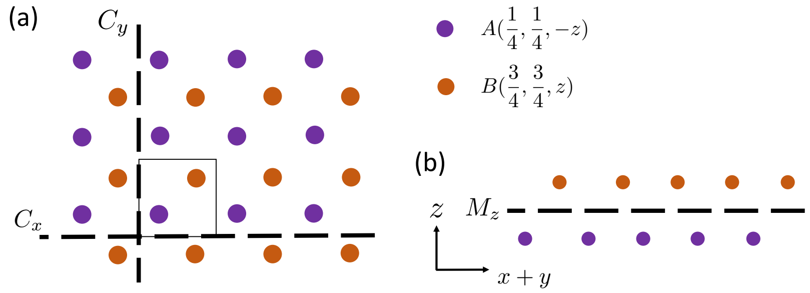


FIG. 1. (a) The top view of the 2D square net lattice. The purple and orange dots denote the $A$ and $B$ sublattices in different $z$ planes. $C_x$ and $C_y$ mark the non-symmorphic rotational symmetries. (b) The side view of the lattice along the $x+y$ direction. $M_z$ denotes the non-symmorphic glide mirror symmetry.

As described in Ref. [1], a combination of the time reversal, inversion, and non-symmorphic symmetries enforces the dimension of the irreducible representation (irrep) and leads to a fourfold degenerate crossing at high symmetry points $X$, $Y$ and $M$ respectively. The present lattice belongs to the layer group $P4/nmm$, with non-symmorphic symmetry $\{M_z|\frac{1}{2}\frac{1}{2}\}$, $\{C_{2x}|\frac{1}{2}0\}$ and $\{C_{2y}|0\frac{1}{2}\}$. It has been proved in Ref. [1] on the original basis that $\{M_z|\frac{1}{2}\frac{1}{2}\}$ and $\{C_{2x}|\frac{1}{2}0\}$ enforce the Dirac points at $X$; $\{M_z|\frac{1}{2}\frac{1}{2}\}$ and $\{C_{2y}|0\frac{1}{2}\}$ enforce the Dirac points at $Y$; $\{C_{2x}|\frac{1}{2}0\}$ and $\{C_{2y}|0\frac{1}{2}\}$ enforce the Dirac points at $M$. Here, we take the $M$ point as an example and exam the stability of $k \cdot p$ theory near it in the newly rotated basis. Near the $k = M$ point,

$$h_0(M + \boldsymbol{q}) = t_{SO}(\tau_z \sigma_y q_x - \tau_z \sigma_x q_y). \tag{S5}$$

In the rotated basis, at $M$, the time-reversal symmetry $\Theta = i\sigma_x K$, the inversion symmetry $P = -\tau_z$. The only allowed mass term is $\tau_z$, while it is forbidden by the non-symmorphic symmetries $\{C_{2x}|\frac{1}{2}0\} = -\tau_y\sigma_y$, $\{C_{2y}|0\frac{1}{2}\} = \tau_y\sigma_x$. Therefore the four-fold Dirac crossing at $M$ is stable.

### A. Minimal interacting model

We introduce four-fermion interactions that preserve the following global symmetries of $h_0$,

- Chiral-$U(1)$: $[h_0(\boldsymbol{k}), e^{i\eta_{\boldsymbol{k}}\tau_3\otimes\sigma_0}] = 0$ with $\eta_{\boldsymbol{k}}$ being an arbitrary $\boldsymbol{k}$-dependent angle;
- Fourfold rotation about $\boldsymbol{k} = 0$: $h_0(\boldsymbol{k}) \to h_0(\boldsymbol{k}') = e^{\frac{i\pi}{4}\tau_3\otimes\sigma_3} h_0(\boldsymbol{k}) e^{-\frac{i\pi}{4}\tau_3\otimes\sigma_3}$,

to obtain

$$\begin{aligned} H_I(\boldsymbol{k}) =& \frac{U_c}{2}\left(\Phi^\dagger_{\boldsymbol{k}}\Phi_{\boldsymbol{k}} - \frac{1}{2}\right)^2 + V_{03}\left(\Phi^\dagger_{\boldsymbol{k}}\tau_0\otimes\sigma_3\Phi_{\boldsymbol{k}}\right)^2 + V_{30}\left(\Phi^\dagger_{\boldsymbol{k}}\tau_3\otimes\sigma_0\Phi_{\boldsymbol{k}}\right)^2 + \frac{U_s}{2}\left(\Phi^\dagger_{\boldsymbol{k}}\tau_3\otimes\sigma_3\Phi_{\boldsymbol{k}}\right)^2 \\ &+ V_1'\left[\left(\Phi^\dagger_{\boldsymbol{k}}\tau_1\otimes\sigma_1\Phi_{\boldsymbol{k}}\right)^2 + \left(\Phi^\dagger_{\boldsymbol{k}}\tau_2\otimes\sigma_1\Phi_{\boldsymbol{k}}\right)^2\right] + V_2'\left[\left(\Phi^\dagger_{\boldsymbol{k}}\tau_1\otimes\sigma_2\Phi_{\boldsymbol{k}}\right)^2 + \left(\Phi^\dagger_{\boldsymbol{k}}\tau_2\otimes\sigma_2\Phi_{\boldsymbol{k}}\right)^2\right], \end{aligned} \tag{S6}$$

where the unitary transfortion between the two bases $\tilde{\Phi}_{\boldsymbol{k}} \to \Phi_{\boldsymbol{k}} = e^{i\frac{\pi}{4}\tau_2\otimes\sigma_3}\tilde{\Phi}_{\boldsymbol{k}}$. $h_0(\boldsymbol{k})$ is diagonalized by the matrix

$$\mathrm{M}_{\boldsymbol{k}} = \begin{pmatrix} e^{\frac{i\varphi_k}{2}}\cos\left(\frac{\vartheta_k}{2}\right) & 0 & ie^{\frac{i\varphi_k}{2}}\sin\left(\frac{\vartheta_k}{2}\right) & 0 \\ ie^{-\frac{1}{2}(i\varphi_k)}\sin\left(\frac{\vartheta_k}{2}\right) & 0 & e^{-\frac{1}{2}(i\varphi_k)}\cos\left(\frac{\vartheta_k}{2}\right) & 0 \\ 0 & ie^{\frac{i\varphi_k}{2}}\sin\left(\frac{\vartheta_k}{2}\right) & 0 & e^{\frac{i\varphi_k}{2}}\cos\left(\frac{\vartheta_k}{2}\right) \\ 0 & e^{-\frac{1}{2}(i\varphi_k)}\cos\left(\frac{\vartheta_k}{2}\right) & 0 & ie^{-\frac{1}{2}(i\varphi_k)}\sin\left(\frac{\vartheta_k}{2}\right) \end{pmatrix} \tag{S7}$$

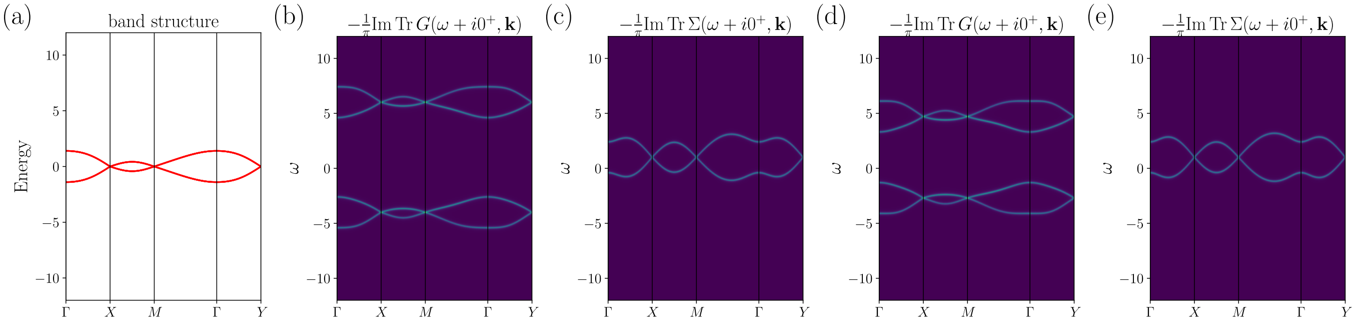


FIG. 2. (a) The band structure of the 2D square net lattice with tight binding parameters $t = 0.7$ and $t_{SO} = 0.42$. (b) The spectral function $A(\omega, \boldsymbol{k}) = -\frac{1}{\pi}\mathrm{Im\ Tr}\ G(\omega + i\delta, \boldsymbol{k})$. Here we choose the Hamiltonian parameters as $U_s = U_c = 5$ and $\mu = 5$. (c) The imaginary part of the retard self energy $\Sigma(\omega + i\delta, \boldsymbol{k})$. A divergent self energy imaginary part indicates a Green's function zero point. Both the spectral function and self energy are evaluated numerically with exact many-body wavefunctions. In subfigures (d) and (e) we also provide the numerical solution to the spectral function and self energy imaginary part with $V_{03} = V_{30} = 0.5$ and $V_1' = V_2' = 0.2$. Although the dispersion of both zeros and poles of the Green's function have been changed, the result is qualitatively similar to the analytical solvable case discussed in the main text.

with $\tan\varphi_{\boldsymbol{k}} = \sin k_x / \sin k_y$ and $\tan\vartheta_{\boldsymbol{k}} = \left(\frac{t_{SO}}{2t}\sqrt{\sin^2 k_x + \sin^2 k_y}\right) / \left(\cos\frac{k_x}{2}\cos\frac{k_y}{2}\right)$, such that

$$\mathrm{M}_{\boldsymbol{k}}^\dagger h_0(\boldsymbol{k})\mathrm{M}_{\boldsymbol{k}} = \sqrt{\left(2t\cos\frac{k_x}{2}\cos\frac{k_y}{2}\right)^2 + t_{SO}^2\left(\sin^2 k_x + \sin^2 k_y\right)}\ \tau_3 \otimes \sigma_0. \tag{S8}$$

Therefore, the 1st and 2nd (3rd and 4th) bands are degenerate in energy. In the band basis, the $V_{00}$ and $V_{30}$ vertices remain momentum-independent, while the rest pick up an implicit $\boldsymbol{k}$-dependence through $\varphi_{\boldsymbol{k}}$ and $\vartheta_{\boldsymbol{k}}$. For example, using $\Psi_{\boldsymbol{k}} = (\psi_{1,\uparrow}, \psi_{1,\downarrow}, \psi_{2,\uparrow}, \psi_{2,\downarrow})_{\boldsymbol{k}}^\intercal$ as a representation of the band basis with $\{\psi_{j,\uparrow}, \psi_{j,\downarrow}\}_{\boldsymbol{k}}$ being degenerate, we obtain

$$\frac{U_s}{2}\left(\Phi_{\boldsymbol{k}}^\dagger \tau_3 \otimes \sigma_3 \Phi_{\boldsymbol{k}}\right)^2 \to \frac{U_s}{2}\left(\cos\vartheta_{\boldsymbol{k}}\ \Psi_{\boldsymbol{k}}^\dagger \tau_3 \otimes \sigma_0 \Psi_{\boldsymbol{k}} - \sin\vartheta_{\boldsymbol{k}}\ \Psi_{\boldsymbol{k}}^\dagger \tau_2 \otimes \sigma_0 \Psi_{\boldsymbol{k}}\right)^2. \tag{S9}$$

The simplest solvable instance of the HK model is obtained in limit $t \gg t_{SO}$ by the switching off all interaction vertices except $U_c$ and $U_s$. Since $\vartheta_k$ remains small throughout the Brillouin zone, except a small $\sim (t_{SO}/t) \ll 1$ neighborhood of the Brillouin zone boundary, we treat the term proportional to $\sin\vartheta_{\boldsymbol{k}}$ in Eq. (S9) as a perturbation. Thus, we obtain a minimal interacting model with,

$$H_I(\boldsymbol{k}) = (U_c + U_s)(n_{1,\uparrow}n_{1,\downarrow} + n_{2,\uparrow}n_{2,\downarrow})_{\boldsymbol{k}} + (U_c - U_s)(n_{1,\uparrow}n_{2,\uparrow} + n_{1,\uparrow}n_{2,\downarrow} + n_{1,\downarrow}n_{2,\uparrow} + n_{1,\downarrow}n_{2,\downarrow})_{\boldsymbol{k}}, \tag{S10}$$

where $n_{j,\sigma}$ is the density operator for the $(j,\sigma)$-th band. In the main text we express $U = (U_c + U_s)$ and $U' = (U_c - U_s)$.

### B. Numerical solution for generic interactions

The $\sin\theta_{\boldsymbol{k}}$-dependent terms in (S9) at more generic ratios of $(t/t_{SO})$ cannot be ignored, and their impact is assessed numerically. Since the interaction terms $H_I$ is local in momentum space, we are able to diagonalize the interacting Hamiltonian for each $\boldsymbol{k}$ and obtain the exact many-body wavefunctions numerically. Therefore, the retarded Green's functions and self-energies can also be solved exactly. We first choose $t = 0.7, t_{SO} = 0.42, U_c = 5.5, U_s = 4.5$ and $\mu = 5$, and solve the retarded Green's functions, the spectral functions and the self energy as functions of $\boldsymbol{k}, \omega$ numerically. In Figs. 2(b-c), we present the spectral function and the *imaginary part* of the retarded self-energy, whose divergence demonstrate the poles and zeros of the Green's function, respectively.

We also consider the effect of the more general set of interactions in (S6) with non-zero values of $V_{03}, V_{30}, V_1'$ and $V_2'$, and present the results in Figs. 2 (d-e). The zeros and poles of the Green's functions are still qualitatively similar to the case discussed in main text, although the dispersion relations of them are different.

| Particle # | States |
|---|---|
| 0 | $\|0\rangle$ |
| 1 | $\|\uparrow 0\rangle$, $\|0\downarrow\rangle$ |
| 2 | $\|\uparrow\downarrow\rangle$ |

TABLE I. List of four possible states with $n = 0, 1, 2$ particles with spin $\sigma$ distributed for a single band with momentum $\boldsymbol{k}$.

| Particle # | States |
|---|---|
| 0 | $\|0\rangle$ |
| 1 | $\|\uparrow;0\rangle, \|\downarrow;0\rangle, \|0;\uparrow\rangle, \|0;\downarrow\rangle$ |
| 2 | $\|\uparrow\downarrow;0\rangle, \|0;\uparrow\downarrow\rangle, \|\uparrow 0;\uparrow 0\rangle$ <br> $\|0\downarrow;0\downarrow\rangle, \|\uparrow 0;0,\downarrow\rangle, \|0\downarrow;\uparrow 0\rangle$ |
| 3 | $\|\uparrow\downarrow;\uparrow 0\rangle, \|\uparrow\downarrow;0\downarrow\rangle, \|\uparrow 0;\uparrow\downarrow\rangle, \|0\downarrow;\uparrow\downarrow\rangle$ |
| 4 | $\|\uparrow\downarrow;\uparrow\downarrow\rangle$ |

TABLE II. List of sixteen possible states with $n = 0, .., 4$ particles with spin $\sigma$ distributed over two bands with momentum $\boldsymbol{k}$. The two bands occupancies are separated by ";".

## II. GREEN'S FUNCTION

In this section, we outline the formulas leading to the expressions for the total Green's functions. The time ordered Green's function is defined in imaginary time by

$$\begin{aligned} G_{\boldsymbol{k}_1\sigma_1\boldsymbol{k}_2\sigma_2}(\tau) &= -\theta(\tau)\langle e^{H\tau}\psi^{\alpha}_{\boldsymbol{k}_1\sigma_1}e^{-H\tau}\psi^{\beta\dagger}_{\boldsymbol{k}_2\sigma_2}\rangle \\ &+ \theta(-\tau)\langle\psi^{\alpha\dagger}_{\boldsymbol{k}_2\sigma_2}e^{H\tau}\psi^{\beta}_{\boldsymbol{k}_1\sigma_1}e^{-H\tau}\rangle. \end{aligned} \tag{S11}$$

The Fourier transform of Green's function in Matsubara frequency space is given by $G(\tau) = \frac{1}{\beta}\sum_n e^{-i\omega_n\tau}G(i\omega_n)$. We can now decompose the propagator in terms of a complete set of eigenstates (listed in Table II) by inserting identities in the definition of $G_{\boldsymbol{k}_1\sigma_1\boldsymbol{k}_2\sigma_2}(\tau)$. Only same spin and momentum transitions are allowed. This gives us the following expression of the total Green's function in terms of a complete set of eigenstates

$$\begin{aligned} \langle e^{H\tau}\psi^{\alpha}_{\boldsymbol{k}_1\sigma_1}e^{-H\tau}\psi^{\beta\dagger}_{\boldsymbol{k}_2\sigma_2}\rangle &= \frac{1}{Z}\sum_{\lambda\lambda'}e^{-\beta E_\lambda}e^{(E_\lambda-E_{\lambda'})\tau} \\ &\quad \langle\lambda|\psi^{\alpha}_{\boldsymbol{k}_1\sigma_1}|\lambda'\rangle\langle\lambda'|\psi^{\beta\dagger}_{\boldsymbol{k}_2\sigma_2}|\lambda\rangle \end{aligned} \tag{S12}$$

$$\begin{aligned} \langle\psi^{\alpha\dagger}_{\boldsymbol{k}_2\sigma_2}e^{H\tau}\psi^{\beta}_{\boldsymbol{k}_1\sigma_1}e^{-H\tau}\rangle &= \frac{1}{Z}\sum_{\lambda\lambda'}e^{-\beta E_\lambda}e^{-(E_\lambda-E_{\lambda'})\tau} \\ &\quad \langle\lambda|\psi^{\alpha\dagger}_{\boldsymbol{k}_2\sigma_2}|\lambda'\rangle\langle\lambda'|\psi^{\beta}_{\boldsymbol{k}_1\sigma_1}|\lambda\rangle. \end{aligned} \tag{S13}$$

Here $Z$ is the total partition function. We can then evaluate the total Fourier transformed interacting Green's function for the first band in the basis of Table II. When $U' \neq 0$, we must evaluate the role of cross terms since we cannot decompose the partition function as a direct product of partition functions for the individual bands. Using the basis in Table II, the new partition function becomes $Z = \prod_{\boldsymbol{k}} Z_{\boldsymbol{k}}$ where

$$Z_{\boldsymbol{k}} = 1 + \sum_{i=1}^{2}\left(2e^{-\beta\xi_i} + e^{-\beta(2\xi_i+U)}\right) + 4e^{-\beta(\xi_1+\xi_2+U')} + 2e^{-\beta(2\xi_1+\xi_2+U+2U')} + 2e^{-\beta(\xi_1+2\xi_2+U+2U')} + e^{-\beta(2\xi_1+2\xi_2+2U+4U')}.$$

In the expression for $Z_{\boldsymbol{k}}$, we have suppressed the momentum argument for convenience of notation. We can then evaluate the total Fourier transformed interacting Green's function for the first band in the basis of Table II as

$$\begin{aligned} Z_{\boldsymbol{k}}G^{(1)}(z) &= \frac{1+e^{-\beta\xi_1}}{z-\xi_1} + e^{-\beta\xi_1}\frac{1+e^{-\beta(\xi_1+U)}}{z-\xi_1-U} + 2e^{-\beta\xi_2}\frac{1+e^{-\beta(\xi_1+U')}}{z-\xi_1-U'} + 2e^{-\beta(\xi_1+\xi_2+U')}\frac{1+e^{-\beta(\xi_1+U+U')}}{z-\xi_1-U-U'} \\ &+ e^{-\beta(2\xi_2+U)}\frac{1+e^{-\beta(\xi_1+2U')}}{z-\xi_1-2U'} + e^{-\beta(\xi_1+2\xi_2+U+2U')}\frac{1+e^{-\beta(\xi_1+U+2U')}}{z-\xi_1-U-2U'}. \end{aligned} \tag{S14}$$

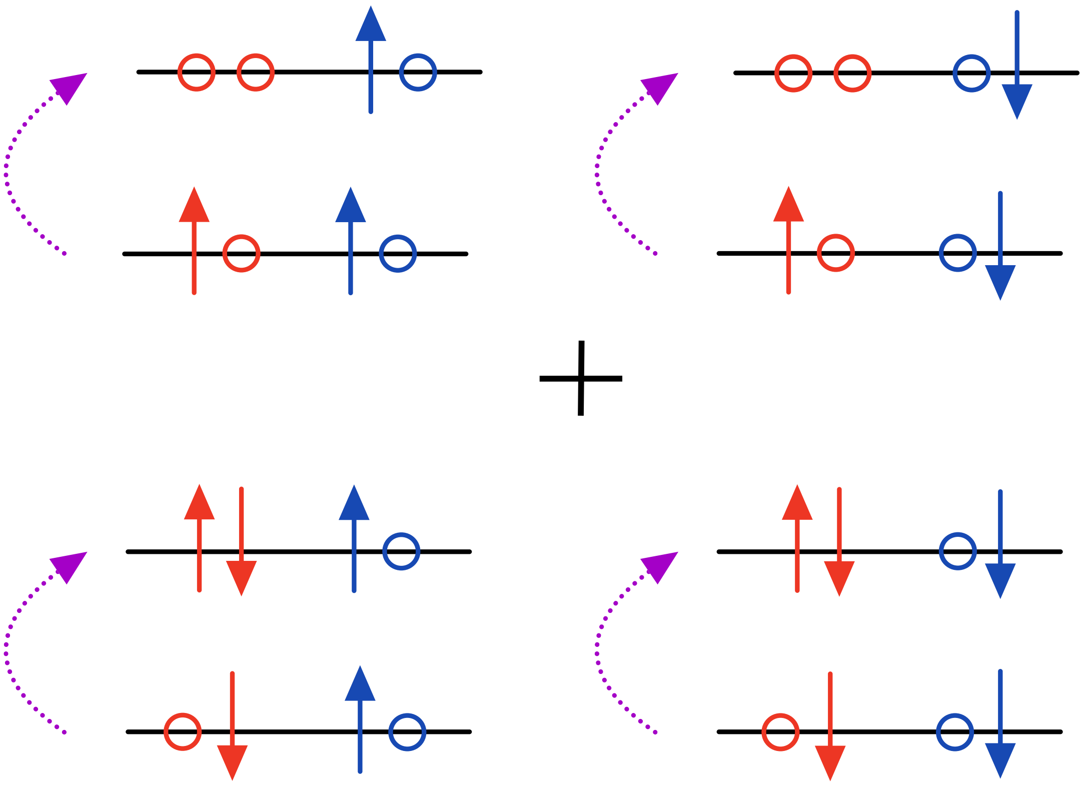

FIG. 3. Transitions contributing to the interacting Green's function in Eq. S14 at a given momentum and zero temperature. The red and blue colors denote the two band degrees of freedom. The circles denote empty states and arrows are pseudo-spin degrees of freedom. The top (bottom) row corresponds to electron removal (addition) states. Their excitation energies are equal and opposite in the presence of time-reversal symmetry. Together, they sum to zero yielding zero surfaces in momentum space.

The Green's function above simplifies in the zero temperature limit where both $\xi_1(\boldsymbol{k}), \xi_2(\boldsymbol{k})$ are filled with $U, U' > 0$. Further when $U + 2U' > |\xi_1| + 2|\xi_2|, 2|\xi_1| + |\xi_2|$ and $U > 2|\xi_1|, 2|\xi_2|$ but $U' < |\xi_1| + |\xi_2|$, the partition function is approximated as $Z_{\boldsymbol{k}} \simeq 4e^{-\beta(\xi_1+\xi_2+U')}$. The Green's function then takes a simple form

$$G^{(1)}(z) = \frac{1}{2}\left[\frac{1}{z - \tilde{\xi}_1 + U/2 - U'} + \frac{1}{z - \tilde{\xi}_1 - U/2 - U'}\right] \tag{S15}$$

with $\tilde{\xi}_i$ being the bare dispersion. Clearly there exist zeros in the Green's function of band $\tilde{\xi}_1(\boldsymbol{k})$ when $z = \tilde{\xi}_1 + U'$. The same argument then holds for the second component of the Green's function, $G^{(2)}(z)$, when $z = \tilde{\xi}_2 + U'$. It is notable that the above derivation for the existence of zeros holds for any $\xi_1, \xi_2$ that satisfy the conditions mentioned above and not specific to Dirac dispersions. In the main text, we use the expressions with $\xi_{1,2}$ replaced by the dispersions of the Young-Kane model.

## III. ONE-BAND HK MODEL

The one-band HK Hamiltonian in momentum space contains two terms

$$H = H_0 + U\sum_{\boldsymbol{k}}\left(n_{\boldsymbol{k}\uparrow} - \frac{1}{2}\right)\left(n_{\boldsymbol{k}\downarrow} - \frac{1}{2}\right), \tag{S16}$$

where $H_0$ is the non-interacting piece and is given by $H_0 = \sum_{\boldsymbol{k}\sigma} \xi_{\boldsymbol{k}\sigma} c^\dagger_{\boldsymbol{k}\sigma} c_{\boldsymbol{k}\sigma}$. The second term is the interacting piece that is made of density operators $n_{\boldsymbol{k}\sigma} = c^\dagger_{\boldsymbol{k}\sigma} c_{\boldsymbol{k}\sigma}$. Here $c^\dagger_{\boldsymbol{k}\sigma}$ creates an electron in momentum $\boldsymbol{k}$ and spin $\sigma$. $U$ is the strength of interaction that is local in momentum space. When Fourier transformed to real space, the interaction

term is non-zero only for electrons that satisfy the zero center of mass condition. A noteworthy property of Eq. S16 is the commutativity between the kinetic and interaction terms as well as particle number conservation for each $\boldsymbol{k}$. This makes the model analytically tractable in contrast to the Hubbard model. The Hilbert space for each momentum $\boldsymbol{k}$ consists of four states shown in Table I. The partition function for the Hamiltonian Eq. S16 is given by $Z = \prod_{\boldsymbol{k}} Z_{\boldsymbol{k}}$ where $Z_{\boldsymbol{k}} = 1 + 2e^{-\beta\xi_{\boldsymbol{k}}} + e^{-\beta(2\xi_{\boldsymbol{k}}+U)}$. The exact interacting Green's function for the single band case is

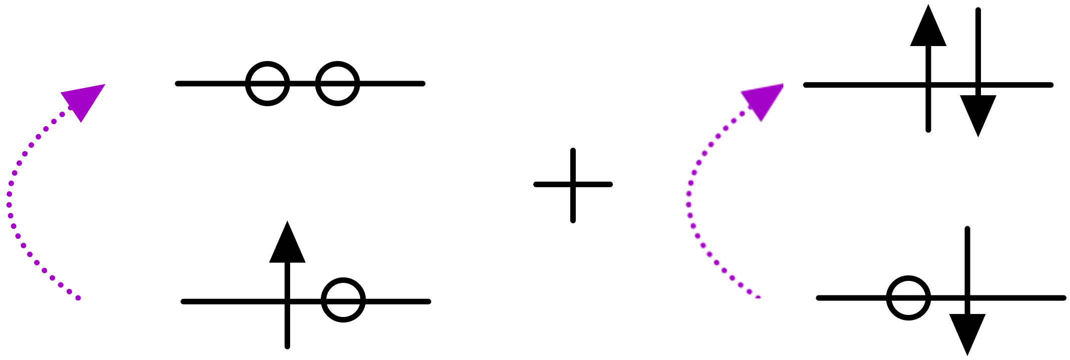

FIG. 4. Single band transitions contributing to the interacting Green's function for a single spin at zero temperature. The circles denote empty states and arrows are pseudo-spin degrees of freedom. The left (right) panel corresponds to electron removal (addition) state. The excitation energies of the two terms are equal and opposite and sum to zero yielding zero surfaces.

$$G_\sigma(\boldsymbol{k}, i\omega_n) = \frac{1 - \langle n_{\boldsymbol{k}} \rangle}{i\omega_n - \xi_{\boldsymbol{k}} - U/2} + \frac{\langle n_{\boldsymbol{k}} \rangle}{i\omega_n - (\xi_{\boldsymbol{k}} - U/2)}. \tag{S17}$$

In the presence of spin-rotation and time reversal invariance, the expression for the Green's function in Eq. S17 is independent of spin. The expectation value $\langle n_{\boldsymbol{k}} \rangle$ is the average occupation of state $\boldsymbol{k}$ and is given by

$$\langle n_{\boldsymbol{k}} \rangle = \frac{e^{-\beta\xi_{\boldsymbol{k}}} + e^{-\beta(2\xi_{\boldsymbol{k}}+U)}}{1 + 2e^{-\beta\xi_{\boldsymbol{k}}} + e^{-\beta(2\xi_{\boldsymbol{k}}+U)}}. \tag{S18}$$

The limit that is of interest to us is $\beta \to \infty$ with $\xi_{\boldsymbol{k}} < 0$ and $U > -\xi_{\boldsymbol{k}}$. In this limit, the partition function is $Z = \prod_{\boldsymbol{k}} 2e^{-\beta\xi_{\boldsymbol{k}}}$ and the the occupation number is $\langle n_{\boldsymbol{k}} \rangle = \frac{1}{2}$. The Green's function then reduces to sum of two terms with equal weight of $\frac{1}{2}$ given by

$$G_\sigma(\boldsymbol{k}, i\omega_n) = \frac{1}{2}\left[\frac{1}{i\omega_n - \xi_{\boldsymbol{k}} - U/2} + \frac{1}{i\omega_n - (\xi_{\boldsymbol{k}} - U/2)}\right]. \tag{S19}$$

The expression in Eq. S19 shows the existence of poles at $i\omega_n = \xi_{\boldsymbol{k}} \pm \frac{U}{2}$ which correspond to the lower and upper Hubbard bands. Importantly, when $i\omega_n = \xi_{\boldsymbol{k}}$, the Green's function is zero; hence, the original contour of poles of the non-interacting system is converted into a contour of zeros of the interacting Green's function. The cancellation of transition amplitudes for the single band case is shown in Fig. 4.

## IV. SPECTRAL DEGENERACY ENFORCED BY NON-SYMMORPHIC CRYSTALLINE SYMMETRY

Here we briefly summarize the formulation of the Green's function based symmetry constraints [2]. This approach starts from expressing the Green's function as a matrix [3–5]. In the space of wavevector $\boldsymbol{k}$, frequency $\omega_n$ and internal (eg., spin, orbital and sublattice) quantum number $a$,

$$[G]_{(a,i\omega_n,\boldsymbol{k}),(b,i\omega_m,\boldsymbol{k}')} = -\langle \psi_{a,i\omega_n,\boldsymbol{k}} \psi^\dagger_{b,i\omega_m,\boldsymbol{k}'} \rangle . \tag{S20}$$

In systems with both space and time translational symmetry, the Green's functions can be block-diagonalized as [2]

$$[G]_{(a,i\omega_m,\boldsymbol{k}),(b,i\omega_n,\boldsymbol{k}')} = \delta_{mn}\delta_{\boldsymbol{k}\boldsymbol{k}'}[G(i\omega_n, \boldsymbol{k})]_{ab}. \tag{S21}$$

Therefore it is enough to consider the Green's functions in each block characterized by $(\omega, \boldsymbol{k})$. We further do the analytical continuation into the real frequency and define $G(\omega, \boldsymbol{k}) = G^R(\omega, \boldsymbol{k}) - G^A(\omega, \boldsymbol{k})$. The matrix $G(\omega, \boldsymbol{k})$ is skew-Hermitian and commutes with the symmetry operators. Therefore we have

$$\sum_b [G(\omega, \boldsymbol{k})]_{ab}[v_{i\omega(\omega,\boldsymbol{k})}]_b = g_i(\omega, \boldsymbol{k})[v_i(\omega, \boldsymbol{k})]_a \tag{S22}$$

where $g_i(\omega, \boldsymbol{k})$ and $[v_i(\omega, \boldsymbol{k})]_b$ are the $i$-th eigenvalues and eigenvectors of each block. At the high symmetry points, the non-symmorphic symmetry further enforces the eigenvectors to form an irrep with a higher dimension [1]. For example, in the case of the 2D square net we considered in the main text, the combination of the time reversal, inversion, and the non-symmorphic glide symmetries enforce the development of the 4d irrep at high symmetry points $X$, $Y$, and $M$. For each $\omega$ at high symmetry points with $\boldsymbol{k} = X, Y, M$, the eigenvalues of Green's function are

$$[G(\omega, \boldsymbol{k})]\Gamma^n(\omega, \boldsymbol{k}) = g(\omega, \boldsymbol{k})\mathbb{1}_{n\times n}\Gamma^n(\omega, \boldsymbol{k}). \tag{S23}$$

where $\Gamma^n$ represents the irrep with dimension $n$. Then, the corresponding spectral functions for each mode in the irrep are identical with

$$\rho(\omega, \boldsymbol{k}) = -\frac{1}{2\pi} g(\omega, \boldsymbol{k}). \tag{S24}$$

## V. MATRIX-FORM OF THE INTERACTING GREEN'S FUNCTION

Here we show that the Green's functions obtained in Eq (6) in the band basis takes the form

$$G(k_0, \boldsymbol{k}) = \frac{1}{\tilde{G}^{-1}(k_0, \boldsymbol{k}) - (U/2)^2 \tilde{G}(k_0, \boldsymbol{k})}, \tag{S25}$$

in the orbital basis, and discuss its consequences. Here, $k_0$ is the Euclidean (equivalently, Matsubara) frequency, and

$$\tilde{G}^{-1}(k_0, \boldsymbol{k}) = ik_0\mathbb{1} - \left[\vec{n}(\boldsymbol{k}) \cdot \vec{\Gamma} - (\mu - U')\mathbb{1}\right] \tag{S26}$$

with $\vec{n}(\boldsymbol{k}) = \left\{-t_{SO}\sin k_y, t_{SO}\sin k_x, 2t\cos\frac{k_x}{2}\cos\frac{k_y}{2}\right\}$, and $\vec{\Gamma} = \tau_3 \otimes \vec{\sigma}$. The net impact of interactions in Eq (3) of the main text is to shift the chemical potential $\mu \to \mu - U'$, and generate the self energy,

$$\Sigma(k_0, \boldsymbol{k}) = (U/2)^2 \tilde{G}(k_0, \boldsymbol{k}). \tag{S27}$$

The poles of $\tilde{G}$ is deduced from the poles of its determinant, which takes the form

$$\det\left\{\tilde{G}\right\} = \frac{1}{\{(k_0 - i(\mu - U'))^2 + |\vec{n}(\boldsymbol{k})|^2\}^2}. \tag{S28}$$

Since $\Sigma \propto \tilde{G}$, the *poles of the self-energy* are twofold degenerate and are located at

$$k_0 = i[(\mu - U') \pm |\vec{n}(\boldsymbol{k})|]. \tag{S29}$$

It is straightforward to be verify that the eigenvalues of $G$ are

$$g_\pm(k_0, \boldsymbol{k}) = \frac{1}{2}\sum_{s=\pm} \frac{1}{ik_0 + \mu - U' \pm |\vec{n}(\boldsymbol{k})| + sU/2}, \tag{S30}$$

which implies,

$$\det\{G\} = \frac{\left\{(k_0 - i(\mu - U'))^2 + |\vec{n}(\boldsymbol{k})|^2\right\}^2}{\left\{(k_0 - i(\mu - U'))^2 + \left(\frac{U}{2} + |\vec{n}(\boldsymbol{k})|\right)^2\right\}^2 \left\{(k_0 - i(\mu - U'))^2 + \left(\frac{U}{2} - |\vec{n}(\boldsymbol{k})|\right)^2\right\}^2}. \tag{S31}$$

Since the numerator of $\det\{G\}$ is precisely equal to the denominator of $\det\left\{\tilde{G}\right\}$, *the zeros of $G$ locate exactly at the poles of $\tilde{G}$.*

Further, $G$ can be brought to the form,

$$G(k_0, \boldsymbol{k}) = iZ_0(k)k_0\mathbb{1} + Z_m u(k)(\mu - U')\mathbb{1} + Z_H(k)\vec{n}(\boldsymbol{k}) \cdot \vec{\Gamma}, \tag{S32}$$

where $Z_x$'s are real-valued functions of $(k_0, \boldsymbol{k})$. Since the terms $\propto \mathbb{1}$ commute with $\Gamma_j$, the eigenvectors of $G(k_0, \boldsymbol{k})$ are entirely determined by $\vec{n}(\boldsymbol{k}) \cdot \vec{\Gamma}$, which is nothing but the single-particle Hamiltonian. Therefore, quite remarkably, *the single-particle Hamiltonian and $G$ share the same eigenstates*, which are independent of $k_0$.

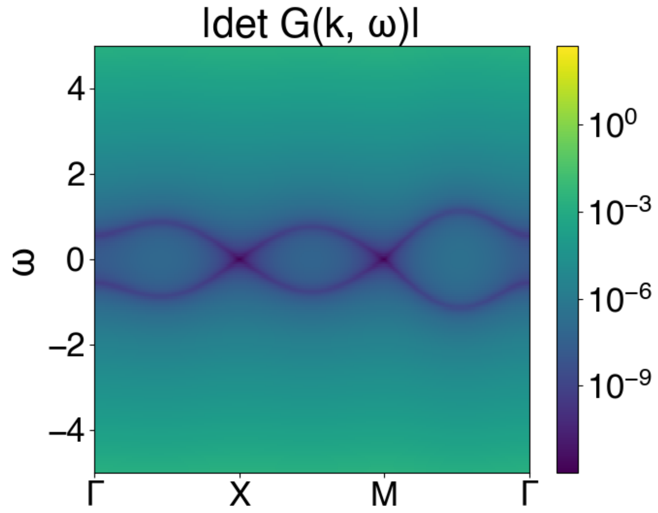


FIG. 5. Plot of the absolute value of the determinant of the single-particle Green's function in the Brillouin zone for the Hubbard model with $(t, t_{SO}, \mu) = (1, 1, 0)$ and $U/t = 14$, which is sufficiently inside the Mott phase. The contours with dark color scale demonstrates the band structure of zeros. The spectral crossings at $X$ and $M$ are protected by lattice symmetries, despite the lack of quasiparticles.

## VI. BROKEN TIME REVERSAL SYMMETRY CASE

Consider the case when a small Zeeman field with strength $h$ splits the bands of the Dirac semimetal into two Weyl cones. Breaking time-reversal symmetry lifts the twofold degeneracy of the bands in the non-interacting limit. In this case, the modified total partition function $Z = \prod_{\boldsymbol{k}} Z_{\boldsymbol{k}}(h)$ and Green's function for the first band are given by

$$\begin{aligned} Z_{\boldsymbol{k}}(h) &= 1 + e^{-\beta\xi_1} + e^{-\beta(\xi_1+h)} + e^{-\beta\xi_2} + e^{-\beta(\xi_2+h)} + e^{-\beta(\xi_1+\xi_2+U')} + 2e^{-\beta(\xi_1+\xi_2+h+U')} + e^{-\beta(\xi_1+\xi_2+2h+U')} \\ &+ e^{-\beta(2\xi_1+h+U)} + e^{-\beta(2\xi_2+h+U)} + e^{-\beta(2\xi_1+\xi_2+U+2U'+h)} + e^{-\beta(2\xi_1+\xi_2+U+2U'+2h)} \\ &+ e^{-\beta(\xi_1+2\xi_2+U+2U'+h)} + e^{-\beta(\xi_1+2\xi_2+U+2U'+2h)} + e^{-\beta(2\xi_1+2\xi_2+2U+4U'+2h)}. \end{aligned} \tag{S33}$$

$$\begin{aligned} Z_{\boldsymbol{k}}(h)G^{(1)}(z,h) &= \frac{1+e^{-\beta\xi_1}}{z-\xi_1} + e^{-\beta(\xi_1+h)}\frac{1+e^{-\beta(\xi_1+U)}}{z-\xi_1-U} + e^{-\beta\xi_2}\frac{1+e^{-\beta(\xi_1+U')}}{z-\xi_1-U'} + e^{-\beta(\xi_2+h)}\frac{1+e^{-\beta(\xi_1+U')}}{z-\xi_1-U'} \\ &+ e^{-\beta(\xi_1+\xi_2+U'+h)}\frac{1+e^{-\beta(\xi_1+U+U')}}{z-\xi_1-U-U'} + e^{-\beta(\xi_1+\xi_2+U'+2h)}\frac{1+e^{-\beta(\xi_1+U+U')}}{z-\xi_1-U-U'} \\ &+ e^{-\beta(2\xi_2+U+h)}\frac{1+e^{-\beta(\xi_1+2U')}}{z-\xi_1-2U'} + e^{-\beta(\xi_1+2\xi_2+U+2U'+2h)}\frac{1+e^{-\beta(\xi_1+U+2U')}}{z-\xi_1-U-2U'}. \end{aligned} \tag{S34}$$

Under the assumptions $\xi_i(\boldsymbol{k}), \xi_2(\boldsymbol{k}) < 0$, $U, U' > 0$, $U+2U' > |\xi_1|+2|\xi_2|, 2|\xi_1|+|\xi_2|$, $U > 2|\xi_1|, 2|\xi_2|$ but $U' < |\xi_1|+|\xi_2|$, the dominant processes contributing to the partition function at zero temperature contain purely inter-band interactions. Further assuming that the magnetic field is small and positive, we have $e^{-\beta(\xi_1+\xi_2+U')} \gg e^{-\beta(\xi_1+\xi_2+h+U')} \gg e^{-\beta(\xi_1+\xi_2+2h+U')}$. As a result, the partition function for momentum $\boldsymbol{k}$ is approximately $Z_{\boldsymbol{k}} \simeq e^{-\beta(\xi_1+\xi_2+U')}$. The Green's function for the $i$-th band reduces to $G^{(i)}(z) = \frac{1}{z-\xi_i-U'}$ hence lacking any zeros. Similarly, when $h < 0$ we have $e^{-\beta(\xi_1+\xi_2+U')} \ll e^{-\beta(\xi_1+\xi_2+h+U')} \ll e^{-\beta(\xi_1+\xi_2+2h+U')}$. The partition function for momentum $\boldsymbol{k}$ is approximately given by $Z_{\boldsymbol{k}} \simeq e^{-\beta(\xi_1+\xi_2+2h+U')}$, and the Green's function reduces to $G^{(i)}(z) = \frac{1}{z-\xi_i-U'-U}$. We can therefore conclude that broken time reversal automatically destroys any zero surfaces. While broken time reversal symmetry can generically remove zeros, the crossings of poles remain protected by symmetry.

## VII. CROSSINGS OF GREEN'S FUNCTION ZEROS FOR THE HUBBARD MODEL

In this section we explicitly demonstrate the symmetry-enforced crossings of Green's function zeros in the Hubbard model,

$$\mathscr{H} = \mathscr{H}_0 + \frac{U}{2}\sum_{i=1,2}\sum_{\boldsymbol{r}}\left(n_{\boldsymbol{r},i,\uparrow} + n_{\boldsymbol{r},i,\downarrow} - 1\right)^2, \tag{S35}$$

via a cluster slave spin calculation (for more details on the method and its application to the class of models discussed here please see [6]). Here, $\mathscr{H}_0$ represents the second quantized form of $h_0$ in Sec. I of the SM. In Fig. 5 we plot the dispersion of the zeros of $G(\omega, \boldsymbol{k})$. The crossings at the high-symmetry points survive the local-in-space interactions of the Hubbard model, and bands of zeros in Figs. 2 of the main text and 5 here agree qualitatively. We note that the cluster slave-spin calculation is designed to capture the zeros of the Greens function. An alternative method is required to access the symmetry-enforced crossings of incoherent spectrum of the Green's function such as those that occur in the Hubbard bands, as discussed in detail in [2].

## VIII. SPECTRAL CROSSINGS ON THE DIAMOND LATTICE

On the diamond lattice the undistorted Fu-Kane-Mele model [7, 8] supports Dirac points at the equivalent $X$ points. The model is given by

$$H_0(\boldsymbol{k}) = \sum_{j=1}^{5} d_j(\boldsymbol{k})\Gamma_j \tag{S36}$$

where $\Gamma_j = \tau_3 \otimes \sigma_j$, $(\Gamma_4, \Gamma_5) = (\tau_2, \tau_1) \otimes \sigma_0$,

$$\begin{aligned}
d_1(\boldsymbol{k}) &= \lambda_{SO}[\sin x_2 - \sin x_3 - \sin(x_2 - x_1) + \sin(x_3 - x_1)] \\
d_2(\boldsymbol{k}) &= \lambda_{SO}[\sin x_3 - \sin x_1 - \sin(x_3 - x_2) + \sin(x_1 - x_2)] \\
d_3(\boldsymbol{k}) &= \lambda_{SO}[\sin x_1 - \sin x_2 - \sin(x_1 - x_3) + \sin(x_2 - x_3)] \\
d_4(\boldsymbol{k}) &= t[\sin x_1 + \sin x_2 + \sin x_3] \\
d_5(\boldsymbol{k}) &= t[1 + \cos x_1 + \cos x_2 + \cos x_3]
\end{aligned} \tag{S37}$$

with

$$(x_1, x_2, x_3) = \left(\frac{k_y + k_z}{2}, \frac{k_x + k_z}{2}, \frac{k_x + k_y}{2}\right). \tag{S38}$$

When both the $t$ and $t_{SO}$ terms are turned on, the band structure of this tight binding model has a Dirac node at the $X$ point in the first Brillouin zone, which has been shown in Fig. 6(a). Similar to Eq. (2) in the main text, we could add a Hatsugai-Kohmoto style interacting Hamiltonian into this model:

$$H = \sum_{\boldsymbol{k}} \mathcal{H}_{\boldsymbol{k}} \tag{S39}$$

$$\mathcal{H}_{\boldsymbol{k}} = \tilde{\Phi}^\dagger_{\boldsymbol{k}}(H_0(\boldsymbol{k}) - \mu\mathbb{1})\tilde{\Phi}_{\boldsymbol{k}} + U_1\left(\tilde{\Phi}^\dagger_{\boldsymbol{k}}\tilde{\Phi}_{\boldsymbol{k}}\right)^2 + U_2\left(\tilde{\Phi}^\dagger_{\boldsymbol{k}}\tau_3 \otimes \sigma_3\tilde{\Phi}_{\boldsymbol{k}}\right)^2 - \frac{U_1 + U_2}{2}\tilde{\Phi}^\dagger_{\boldsymbol{k}}\tilde{\Phi}_{\boldsymbol{k}}, \tag{S40}$$

in which $\tilde{\Phi}^\intercal_{\boldsymbol{k}} = (\phi_{1\uparrow\boldsymbol{k}}, \phi_{1\downarrow\boldsymbol{k}}, \phi_{2\uparrow\boldsymbol{k}}, \phi_{2\downarrow\boldsymbol{k}})$ represents the spin and orbital basis. Since the interaction is local in the momentum space, we expect the dispersive zeros and poles will exist with a suffiently large $U_1$ and $U_2$. We choose the values of interaction $U_1 = U_2 = 5$ and chemical potential $\mu = 5$, and numerically solve the Green's functions of this model. The spectral function and the imaginary part of the self-energy are shown in Fig. 6(b-c), which indicate the dispersion of the poles and zeros of the Green's function, respectively.

⊕ csetty@rice.edu
† shouvik.sur@rice.edu
* These authors contributed equally

[1] Steve M Young and Charles L Kane, "Dirac semimetals in two dimensions," Phys. Rev. Lett. **115**, 126803 (2015).

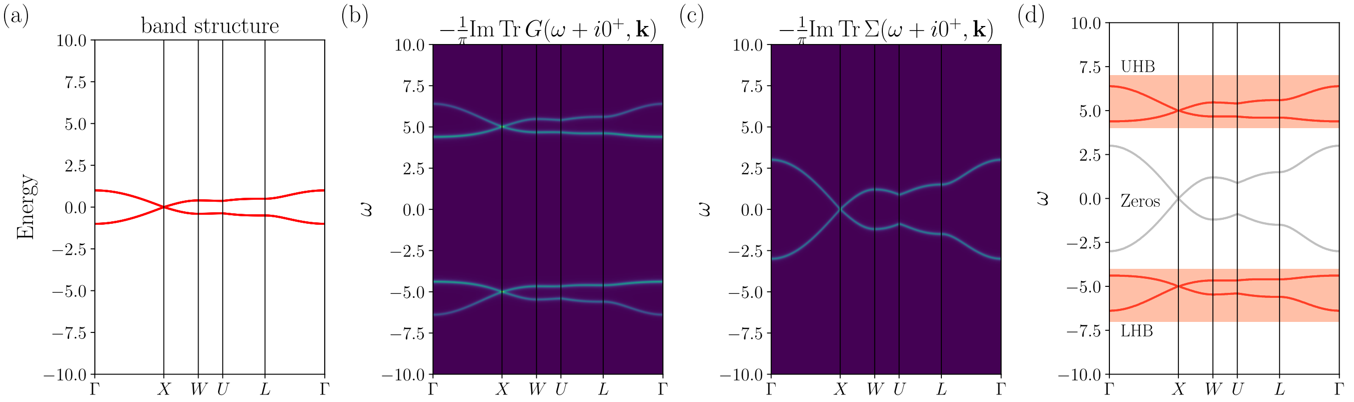


FIG. 6. (a) The band structure of the diamond lattice with $t = 0.25$ and $\lambda_{SO} = 0.1$. (b) The spectral function $A(\omega, \boldsymbol{k})$ of the $U_1 = U_2 = 5$ and $\mu = 5$. (c) The imaginary part of the retarded self-energy. (d) Dispersion of the zeros and poles of the Green's function, and the upper/lower Hubbard bands are labeled by orange shaded regions.


[2] Haoyu Hu Hu, Lei Chen, Chandan Setty, Mikel Garcia-Diez, Sarah E Grefe, Xinlin Yan, Monika Lužnik, Nikolas Reumann, Andrey Prokofiev, Stefan Kirchner, Maia G. Vergniory, Silke Paschen, Jennifer Cano, and Qimiao Si, "Topological semimetals without quasiparticles," arXiv preprint arXiv:2110.06182 (2021).

[3] Aleksei Alekseevich Abrikosov, Lev Petrovich Gorkov, and Igor Ekhielevich Dzyaloshinski, *Methods of quantum field theory in statistical physics* (Courier Corporation, 2012).

[4] V. Gurarie, "Single-particle Green's functions and interacting topological insulators," Phys. Rev. B **83**, 085426 (2011).

[5] Zhong Wang, Xiao-Liang Qi, and Shou-Cheng Zhang, "Topological invariants for interacting topological insulators with inversion symmetry," Phys. Rev. B **85**, 165126 (2012).

[6] Lei Chen, Haoyu Hu, Maia G Vergniory, Jennifer Cano, and Qimiao Si, "Dirac zeros in an orbital selective Mott phase: Green's function berry curvature and flux quantization," arXiv preprint arXiv:2401.12156 (2024).

[7] Liang Fu, Charles L Kane, and Eugene J Mele, "Topological insulators in three dimensions," Phys. Rev. Lett. **98**, 106803 (2007).

[8] Liang Fu and Charles L Kane, "Topological insulators with inversion symmetry," Phys. Rev. B **76**, 045302 (2007).
